# Supplementary material for: Fast Monte Carlo Rendering via Multi-Resolution Sampling
Source: arXiv:2106.12802 source file (2021-06-24)
Supplement: Supplementary file 1 [file appendix.tex]

\appendix

\begin{center}
    \Large \textbf{Appendix}
\end{center}

\section{Additional Blender Cycles Ray-tracing(BCR) Dataset Details}
Blender Cycles Ray-tracing (BCR) dataset consists of a large number of high quality ray-tracing images. It covers a variety of scene contents, such as indoor, outdoor, landscapes, fruits, plants, vehicles, animals, glass, and science fiction objects. For each image, we not only provide the final rendered image but also the render layers, which is essential for Monte Carlo rendering. Our layers include 
\emph{AO},
\emph{Debug Render Time},
\emph{Denoising Albedo},
\emph{Denoising Depth},
\emph{Denoising Intensity},
\emph{Denoising Normal},
\emph{Denoising Shadowing},
\emph{Denoising Variance},
\emph{Depth},
\emph{DiffCol},
\emph{DiffDir},
\emph{DiffInd},
\emph{Emit},
\emph{Env},
\emph{GlossCol},
\emph{GlossDir},
\emph{GlossInd},
\emph{IndexMA},
\emph{IndexOB},
\emph{Mist},
\emph{Noisy Image},
\emph{Normal},
\emph{Shadow},
\emph{SubsurfaceCol},
\emph{SubsurfaceDir},
\emph{SubsurfaceInd},
\emph{TransCol},
\emph{TransDir},
\emph{TransInd},
\emph{UV},
\emph{Vector},
\emph{VolumeDir}, and
\emph{VolumeInd}. Figure~\ref{fig:layers3} shows the visual examples of render layers. To visualize these layers,  we convert the HR image to sRGB space. For depth, we shows $1/(I_{Depth} + 0.00001)$.

\section{Additional Examples from the Gharbi dataset}
In Figure~\ref{fig:comp_pbrt}, we provide more visual examples on the Gharbi dataset~\cite{gharbi2019sample}. Our methods are able to generate high quality rendering results. Although our RelMSE score is higher than Gharbi~\cite{gharbi2019sample}, our  results look more plausible. For instance, the pink desktop in the fourth example is flat. Although our RelMSE is $10\times$ higher, our prediction contains much fewer artifacts compared to Gharbi. Our method failed to recover all these values because (1) our method is trained on the BCR dataset which is rendered by a different renderer, Cycles (2) to run our method on the Gharbi dataset, we set the variance layer of our input to the constant 1, as the variance layer of BCR has a different format with the one of Gharbi dataset.

\begin{figure*}[tb]
    % \newlength\indentspace
    \setlength{\indentspace}{-3.5mm}
    \newcommand{\layersubfigsize}{0.17}
    \scriptsize
    \centering
        \begin{adjustbox}{valign=t}
        \tiny
            \begin{tabular}{ccccc}
                \includegraphics[width=\layersubfigsize\textwidth]{fig/pass/68819_Seen_in_a_Restaurant_oil-vinegar.001_RenderLayer.Combined.png} \hspace{\indentspace} &
                \includegraphics[width=\layersubfigsize\textwidth]{fig/pass/68819_Seen_in_a_Restaurant_oil-vinegar.001_RenderLayer.AO.png} \hspace{\indentspace} &
                \includegraphics[width=\layersubfigsize\textwidth]{fig/pass/68819_Seen_in_a_Restaurant_oil-vinegar.001_RenderLayer.Denoising Albedo.png} \hspace{\indentspace} &
                \includegraphics[width=\layersubfigsize\textwidth]{fig/pass/68819_Seen_in_a_Restaurant_oil-vinegar.001_RenderLayer.Denoising Depth.png} \hspace{\indentspace} &
                \includegraphics[width=\layersubfigsize\textwidth]{fig/pass/68819_Seen_in_a_Restaurant_oil-vinegar.001_RenderLayer.Denoising Normal.png} 
                \\
                HR \hspace{\indentspace} &
                AO \hspace{\indentspace} &
                Denoising Albedo \hspace{\indentspace}&
                Denoising Depth \hspace{\indentspace}&
                Denoising Normal
                \\
                \includegraphics[width=\layersubfigsize\textwidth]{fig/pass/68819_Seen_in_a_Restaurant_oil-vinegar.001_RenderLayer.Denoising Shadowing.png} \hspace{\indentspace} &
                \includegraphics[width=\layersubfigsize\textwidth]{fig/pass/68819_Seen_in_a_Restaurant_oil-vinegar.001_RenderLayer.Denoising Variance.png} \hspace{\indentspace} &
                \includegraphics[width=\layersubfigsize\textwidth]{fig/pass/68819_Seen_in_a_Restaurant_oil-vinegar.001_RenderLayer.Depth.png} \hspace{\indentspace} &
                \includegraphics[width=\layersubfigsize\textwidth]{fig/pass/68819_Seen_in_a_Restaurant_oil-vinegar.001_RenderLayer.DiffCol.png} \hspace{\indentspace} &
                \includegraphics[width=\layersubfigsize\textwidth]{fig/pass/68819_Seen_in_a_Restaurant_oil-vinegar.001_RenderLayer.DiffDir.png}
                \\
                Denoising Shadowing \hspace{\indentspace} &
                Denoising Variance \hspace{\indentspace}&
                Depth  \hspace{\indentspace} &
                DiffCol \hspace{\indentspace} &
                DiffDir
                \\
                \includegraphics[width=\layersubfigsize\textwidth]{fig/pass/68819_Seen_in_a_Restaurant_oil-vinegar.001_RenderLayer.DiffInd.png} \hspace{\indentspace} &
                \includegraphics[width=\layersubfigsize\textwidth]{fig/pass/68819_Seen_in_a_Restaurant_oil-vinegar.001_RenderLayer.Emit.png} \hspace{\indentspace} &
                \includegraphics[width=\layersubfigsize\textwidth]{fig/pass/68819_Seen_in_a_Restaurant_oil-vinegar.001_RenderLayer.GlossCol.png} \hspace{\indentspace} &
                \includegraphics[width=\layersubfigsize\textwidth]{fig/pass/68819_Seen_in_a_Restaurant_oil-vinegar.001_RenderLayer.GlossDir.png} \hspace{\indentspace} &
                \includegraphics[width=\layersubfigsize\textwidth]{fig/pass/68819_Seen_in_a_Restaurant_oil-vinegar.001_RenderLayer.GlossInd.png}
                \\
                DiffInd \hspace{\indentspace}&
                Emit  \hspace{\indentspace}&
                GlossCol \hspace{\indentspace} &
                GlossDir \hspace{\indentspace} &
                GlossInd
                \\

                \includegraphics[width=\layersubfigsize\textwidth]{fig/pass/68819_Seen_in_a_Restaurant_oil-vinegar.001_RenderLayer.IndexMA.png}  \hspace{\indentspace} &
                 \includegraphics[width=\layersubfigsize\textwidth]{fig/pass/68819_Seen_in_a_Restaurant_oil-vinegar.001_RenderLayer.SubsurfaceCol.png} \hspace{\indentspace} &
                \includegraphics[width=\layersubfigsize\textwidth]{fig/pass/68819_Seen_in_a_Restaurant_oil-vinegar.001_RenderLayer.SubsurfaceDir.png} \hspace{\indentspace} &
                \includegraphics[width=\layersubfigsize\textwidth]{fig/pass/68819_Seen_in_a_Restaurant_oil-vinegar.001_RenderLayer.SubsurfaceInd.png} \hspace{\indentspace} &
                \includegraphics[width=\layersubfigsize\textwidth]{fig/pass/68819_Seen_in_a_Restaurant_oil-vinegar.001_RenderLayer.UV.png} 
                \\
                IndexMA  \hspace{\indentspace}&
                SubsurfaceCol \hspace{\indentspace} &
                SubsurfaceDir \hspace{\indentspace} &
                SubsurfaceInd \hspace{\indentspace}&
                UV 
                \\
                \includegraphics[width=\layersubfigsize\textwidth]{fig/pass/68819_Seen_in_a_Restaurant_oil-vinegar.001_RenderLayer.TransCol.png} \hspace{\indentspace} &
                \includegraphics[width=\layersubfigsize\textwidth]{fig/pass/68819_Seen_in_a_Restaurant_oil-vinegar.001_RenderLayer.TransDir.png} \hspace{\indentspace} &
                \includegraphics[width=\layersubfigsize\textwidth]{fig/pass/68819_Seen_in_a_Restaurant_oil-vinegar.001_RenderLayer.TransInd.png} \hspace{\indentspace} &
                \includegraphics[width=\layersubfigsize\textwidth]{fig/pass/68819_Seen_in_a_Restaurant_oil-vinegar.001_RenderLayer.Mist.png}  \hspace{\indentspace} &
                \includegraphics[width=\layersubfigsize\textwidth]{fig/pass/68819_Seen_in_a_Restaurant_oil-vinegar.001_RenderLayer.Normal.png}
                \\
                TransCol \hspace{\indentspace} &
                TransDir \hspace{\indentspace} &
                TransInd \hspace{\indentspace}&
                Mist \hspace{\indentspace} &
                Normal 
                \\
                \includegraphics[width=\layersubfigsize\textwidth]{fig/pass/68819_Seen_in_a_Restaurant_oil-vinegar.001_RenderLayer.Shadow.png} \hspace{\indentspace} &
                \includegraphics[width=\layersubfigsize\textwidth]{fig/pass/68819_Seen_in_a_Restaurant_oil-vinegar.001_RenderLayer.VolumeDir.png} \hspace{\indentspace} &
                \includegraphics[width=\layersubfigsize\textwidth]{fig/pass/68819_Seen_in_a_Restaurant_oil-vinegar.001_RenderLayer.VolumeInd.png} \hspace{\indentspace} &
                \includegraphics[width=\layersubfigsize\textwidth]{fig/pass/68819_Seen_in_a_Restaurant_oil-vinegar.001_RenderLayer.Denoising Intensity.png}\hspace{\indentspace} &
                \includegraphics[width=\layersubfigsize\textwidth]{fig/pass/68819_Seen_in_a_Restaurant_oil-vinegar.001_RenderLayer.Debug Render Time.png}
                \\
                Shadow \hspace{\indentspace} &
                VolumeDir \hspace{\indentspace} &
                VolumeInd \hspace{\indentspace} &
                Denoising Intensity \hspace{\indentspace} &
                Debug Render Time
                \\
                \includegraphics[width=\layersubfigsize\textwidth]{fig/pass/68819_Seen_in_a_Restaurant_oil-vinegar.001_RenderLayer.Env.png} \hspace{\indentspace} &
                \includegraphics[width=\layersubfigsize\textwidth]{fig/pass/68819_Seen_in_a_Restaurant_oil-vinegar.001_RenderLayer.IndexOB.png}\hspace{\indentspace} &
                \includegraphics[width=\layersubfigsize\textwidth]{fig/pass/68819_Seen_in_a_Restaurant_oil-vinegar.001_RenderLayer.Vector.png}\hspace{\indentspace} &
                \includegraphics[width=\layersubfigsize\textwidth]{fig/pass/68819_Seen_in_a_Restaurant_oil-vinegar.001_RenderLayer.Noisy Image.png}\hspace{\indentspace} &
                \\
                Env \hspace{\indentspace} &
                IndexOB \hspace{\indentspace} &
                Vector \hspace{\indentspace} &
                Noisy Image 
                \\
            \end{tabular}
        \end{adjustbox} 
        
        \vspace{-0.1in}
    \caption{Visual examples of the render layers.
    }\vspace{-0.1in}
\label{fig:layers3}
\end{figure*}

\begin{figure*}[t]
    \newlength\indentspace
    \newcommand{\subghafigsize}{0.148}
    \setlength{\indentspace}{-4mm}
    \centering
    \begin{tabular}{cc}
    \hspace{-5.4mm}
        \begin{adjustbox}{valign=t}
        \scriptsize
            \begin{tabular}{c}
              \includegraphics[width=0.24\textwidth]{fig/comp_sbmc/anim-bluespheres_spp_4/masked_gt.png}
                \\
                anim-bluespheres
            \end{tabular}
        \end{adjustbox}
        \hspace{-8.5mm}
        &
        \begin{adjustbox}{valign=t}
        \scriptsize
            \begin{tabular}{ccccc}
                \includegraphics[width=\subghafigsize\textwidth]{fig/comp_sbmc/anim-bluespheres_spp_4//gt.png} \hspace{\indentspace} &
                \includegraphics[width=\subghafigsize\textwidth]{fig/comp_sbmc/anim-bluespheres_spp_4/input.png} \hspace{\indentspace} &
                \includegraphics[width=\subghafigsize\textwidth]{fig/comp_sbmc/anim-bluespheres_spp_4//2011_sen_rpf.png} \hspace{\indentspace} &
                \includegraphics[width=\subghafigsize\textwidth]{fig/comp_sbmc/anim-bluespheres_spp_4/2012_rousselle_nlm.png} \hspace{\indentspace} &
                \includegraphics[width=\subghafigsize\textwidth]{fig/comp_sbmc/anim-bluespheres_spp_4/2015_kalantari_lbf.png} 
                \\
                Ground Truth \hspace{\indentspace} &
                4spp\hspace{\indentspace} &
                Sen~\cite{sen2012filtering} \hspace{\indentspace} &
                Rousselle~\cite{rousselle2011adaptive} \hspace{\indentspace} &
                Kalantari~\cite{kalantari2015machine}
                \\
                PSNR$\uparrow$/RelMSE$\downarrow$ \hspace{\indentspace} &
                18.99/0.4906 \hspace{\indentspace} &
                27.71/0.1153 \hspace{\indentspace} &
                31.67/0.0139 \hspace{\indentspace} &
                33.45/0.0067 
                \\
                \includegraphics[width=\subghafigsize\textwidth]{fig/comp_sbmc/anim-bluespheres_spp_4/2016_bitterli_nfor.png} \hspace{\indentspace} &
                \includegraphics[width=\subghafigsize\textwidth]{fig/comp_sbmc/anim-bluespheres_spp_4/2017_bako_kpcn.png} \hspace{\indentspace} &
                \includegraphics[width=\subghafigsize\textwidth]{fig/comp_sbmc/anim-bluespheres_spp_4/disney_samples_ft.png} \hspace{\indentspace} &
                \includegraphics[width=\subghafigsize\textwidth]{fig/comp_sbmc/anim-bluespheres_spp_4/rmse_multisteps3.png} \hspace{\indentspace} &
                \includegraphics[width=\subghafigsize\textwidth]{fig/comp_sbmc/anim-bluespheres_spp_4/lr_sp_8_lsp_sp_2x2.png}
                \\ 
                Bitterli~\cite{bitterli2016nonlinearly} \hspace{\indentspace} &
                KPCN~\cite{bako2017kernel} \hspace{\indentspace} &
                KPCN-ft~\cite{bako2017kernel} \hspace{\indentspace} &
                Gharbi~\cite{gharbi2019sample} \hspace{\indentspace} &
                Ours $\times2$
                \\
                32.53/0.0092 \hspace{\indentspace} &
                32.32/0.0096 \hspace{\indentspace} &
                30.84/0.0073 \hspace{\indentspace} &
                35.72/\textbf{0.0028} \hspace{\indentspace} &
                \textbf{35.99}/0.0034
                \\
            \end{tabular}
        \end{adjustbox} 
        \\
        \hspace{-5.4mm} 
        \begin{adjustbox}{valign=t}
        \scriptsize
            \begin{tabular}{c}
              \includegraphics[width=0.24\textwidth]{fig/comp_sbmc/AreaLightTestSynthesizer_15_spp_4/masked_gt.png}
                \\
                AreaLightTestSynthesizer\_15
            \end{tabular}
        \end{adjustbox}
        \hspace{-8.5mm}
        &
        \begin{adjustbox}{valign=t}
        \scriptsize
            \begin{tabular}{ccccc}
                \includegraphics[width=\subghafigsize\textwidth]{fig/comp_sbmc/AreaLightTestSynthesizer_15_spp_4/gt.png} \hspace{\indentspace} &
                \includegraphics[width=\subghafigsize\textwidth]{fig/comp_sbmc/AreaLightTestSynthesizer_15_spp_4/input.png} \hspace{\indentspace} &
                \includegraphics[width=\subghafigsize\textwidth]{fig/comp_sbmc/AreaLightTestSynthesizer_15_spp_4/2011_sen_rpf.png} \hspace{\indentspace} &
                \includegraphics[width=\subghafigsize\textwidth]{fig/comp_sbmc/AreaLightTestSynthesizer_15_spp_4/2012_rousselle_nlm.png} \hspace{\indentspace} &
                \includegraphics[width=\subghafigsize\textwidth]{fig/comp_sbmc/AreaLightTestSynthesizer_15_spp_4/2015_kalantari_lbf.png} 
                \\
                Ground Truth \hspace{\indentspace} &
                4spp\hspace{\indentspace} &
                Sen~\cite{sen2012filtering} \hspace{\indentspace} &
                Rousselle~\cite{rousselle2011adaptive} \hspace{\indentspace} &
                Kalantari~\cite{kalantari2015machine}
                \\
                PSNR$\uparrow$/RelMSE$\downarrow$ \hspace{\indentspace} &
                22.78/0.1003 \hspace{\indentspace} &
                33.79/0.0074 \hspace{\indentspace} &
                41.18/0.0035 \hspace{\indentspace} &
                41.36/0.0026
                \\
                \includegraphics[width=\subghafigsize\textwidth]{fig/comp_sbmc/AreaLightTestSynthesizer_15_spp_4/2016_bitterli_nfor.png} \hspace{\indentspace} &
                \includegraphics[width=\subghafigsize\textwidth]{fig/comp_sbmc/AreaLightTestSynthesizer_15_spp_4/2017_bako_kpcn.png} \hspace{\indentspace} &
                \includegraphics[width=\subghafigsize\textwidth]{fig/comp_sbmc/AreaLightTestSynthesizer_15_spp_4/disney_samples_ft.png} \hspace{\indentspace} &
                \includegraphics[width=\subghafigsize\textwidth]{fig/comp_sbmc/AreaLightTestSynthesizer_15_spp_4/rmse_multisteps3.png} \hspace{\indentspace} &
                \includegraphics[width=\subghafigsize\textwidth]{fig/comp_sbmc/AreaLightTestSynthesizer_15_spp_4/lr_sp_8_lsp_sp_2x2.png}
                \\ 
                Bitterli~\cite{bitterli2016nonlinearly} \hspace{\indentspace} &
                KPCN~\cite{bako2017kernel} \hspace{\indentspace} &
                KPCN-ft~\cite{bako2017kernel} \hspace{\indentspace} &
                Gharbi~\cite{gharbi2019sample} \hspace{\indentspace} &
                Ours $\times2$
                \\
                33.83/0.0065 \hspace{\indentspace} &
                39.56/0.0279 \hspace{\indentspace} &
                37.74/0.0046 \hspace{\indentspace} &
                40.69/\textbf{0.0023} \hspace{\indentspace} &
                \textbf{43.20}/0.0037
                \\
            \end{tabular}
        \end{adjustbox} 
        \\
        \hspace{-5.4mm} 
        \begin{adjustbox}{valign=t}
        \scriptsize
            \begin{tabular}{c}
              \includegraphics[width=0.24\textwidth]{fig/comp_sbmc/coffee_spp_4/masked_gt.png}
                \\
                coffee
            \end{tabular}
        \end{adjustbox}
        \hspace{-8.5mm}
        &
        \begin{adjustbox}{valign=t}
        \scriptsize
            \begin{tabular}{ccccc}
                \includegraphics[width=\subghafigsize\textwidth]{fig/comp_sbmc/coffee_spp_4/gt.png} \hspace{\indentspace} &
                \includegraphics[width=\subghafigsize\textwidth]{fig/comp_sbmc/coffee_spp_4/input.png} \hspace{\indentspace} &
                \includegraphics[width=\subghafigsize\textwidth]{fig/comp_sbmc/coffee_spp_4/2011_sen_rpf.png} \hspace{\indentspace} &
                \includegraphics[width=\subghafigsize\textwidth]{fig/comp_sbmc/coffee_spp_4/2012_rousselle_nlm.png} \hspace{\indentspace} &
                \includegraphics[width=\subghafigsize\textwidth]{fig/comp_sbmc/coffee_spp_4/2015_kalantari_lbf.png} 
                \\
                Ground Truth \hspace{\indentspace} &
                4spp\hspace{\indentspace} &
                Sen~\cite{sen2012filtering} \hspace{\indentspace} &
                Rousselle~\cite{rousselle2011adaptive} \hspace{\indentspace} &
                Kalantari~\cite{kalantari2015machine}
                \\
                PSNR$\uparrow$/RelMSE$\downarrow$ \hspace{\indentspace} &
                18.57/1.1857 \hspace{\indentspace} &
                28.99/0.0535 \hspace{\indentspace} &
                21.23/0.8275 \hspace{\indentspace} &
                29.89/0.2450 
                \\
                \includegraphics[width=\subghafigsize\textwidth]{fig/comp_sbmc/coffee_spp_4/2016_bitterli_nfor.png} \hspace{\indentspace} &
                \includegraphics[width=\subghafigsize\textwidth]{fig/comp_sbmc/coffee_spp_4/2017_bako_kpcn.png} \hspace{\indentspace} &
                \includegraphics[width=\subghafigsize\textwidth]{fig/comp_sbmc/coffee_spp_4/disney_samples_ft.png} \hspace{\indentspace} &
                \includegraphics[width=\subghafigsize\textwidth]{fig/comp_sbmc/coffee_spp_4/rmse_multisteps3.png} \hspace{\indentspace} &
                \includegraphics[width=\subghafigsize\textwidth]{fig/comp_sbmc/coffee_spp_4/lr_sp_8_lsp_sp_2x2.png}
                \\ 
                Bitterli~\cite{bitterli2016nonlinearly} \hspace{\indentspace} &
                KPCN~\cite{bako2017kernel} \hspace{\indentspace} &
                KPCN-ft~\cite{bako2017kernel} \hspace{\indentspace} &
                Gharbi~\cite{gharbi2019sample} \hspace{\indentspace} &
                Ours $\times2$
                \\
                24.80/5.4576 \hspace{\indentspace} &
                29.12/0.2789 \hspace{\indentspace} &
                30.12/0.1629 \hspace{\indentspace} &
                31.82/\textbf{0.0349} \hspace{\indentspace} &
                \textbf{32.94}/0.0766
                \\
            \end{tabular}
        \end{adjustbox} 
        \\
        \hspace{-5.4mm} 
        \begin{adjustbox}{valign=t}
        \scriptsize
            \begin{tabular}{c}
              \includegraphics[width=0.24\textwidth]{fig/comp_sbmc/teapot-area-light_spp_4/masked_gt.png}
                \\
                teapot-area-light
            \end{tabular}
        \end{adjustbox}
        \hspace{-8.5mm}
        &
        \begin{adjustbox}{valign=t}
        \scriptsize
            \begin{tabular}{ccccc}
                \includegraphics[width=\subghafigsize\textwidth]{fig/comp_sbmc/teapot-area-light_spp_4/gt.png} \hspace{\indentspace} &
                \includegraphics[width=\subghafigsize\textwidth]{fig/comp_sbmc/teapot-area-light_spp_4/input.png} \hspace{\indentspace} &
                \includegraphics[width=\subghafigsize\textwidth]{fig/comp_sbmc/teapot-area-light_spp_4/2011_sen_rpf.png} \hspace{\indentspace} &
                \includegraphics[width=\subghafigsize\textwidth]{fig/comp_sbmc/teapot-area-light_spp_4/2012_rousselle_nlm.png} \hspace{\indentspace} &
                \includegraphics[width=\subghafigsize\textwidth]{fig/comp_sbmc/teapot-area-light_spp_4/2015_kalantari_lbf.png} 
                \\
                Ground Truth \hspace{\indentspace} &
                4spp\hspace{\indentspace} &
                Sen~\cite{sen2012filtering} \hspace{\indentspace} &
                Rousselle~\cite{rousselle2011adaptive} \hspace{\indentspace} &
                Kalantari~\cite{kalantari2015machine}
                \\
                PSNR$\uparrow$/RelMSE$\downarrow$ \hspace{\indentspace} &
                22.55/0.0976 \hspace{\indentspace} &
                38.52/0.0046 \hspace{\indentspace} &
                42.86/0.0030 \hspace{\indentspace} &
                38.46/0.0041 
                \\
                \includegraphics[width=\subghafigsize\textwidth]{fig/comp_sbmc/teapot-area-light_spp_4/2016_bitterli_nfor.png} \hspace{\indentspace} &
                \includegraphics[width=\subghafigsize\textwidth]{fig/comp_sbmc/teapot-area-light_spp_4/2017_bako_kpcn.png} \hspace{\indentspace} &
                \includegraphics[width=\subghafigsize\textwidth]{fig/comp_sbmc/teapot-area-light_spp_4/disney_samples_ft.png} \hspace{\indentspace} &
                \includegraphics[width=\subghafigsize\textwidth]{fig/comp_sbmc/teapot-area-light_spp_4/rmse_multisteps3.png} \hspace{\indentspace} &
                \includegraphics[width=\subghafigsize\textwidth]{fig/comp_sbmc/teapot-area-light_spp_4/lr_sp_8_lsp_sp_2x2.png}
                \\ 
                Bitterli~\cite{bitterli2016nonlinearly} \hspace{\indentspace} &
                KPCN~\cite{bako2017kernel} \hspace{\indentspace} &
                KPCN-ft~\cite{bako2017kernel} \hspace{\indentspace} &
                Gharbi~\cite{gharbi2019sample} \hspace{\indentspace} &
                Ours $\times2$
                \\
                29.21/14.2664 \hspace{\indentspace} &
                39.27/0.0134 \hspace{\indentspace} &
                38.61/0.0028 \hspace{\indentspace} &
                40.86/\textbf{0.0020} \hspace{\indentspace} &
                \textbf{43.04}/0.0288
                \\
            \end{tabular}
        \end{adjustbox} 
        \\
        \hspace{-5.4mm} 
        \begin{adjustbox}{valign=t}
        \scriptsize
            \begin{tabular}{c}
              \includegraphics[width=0.24\textwidth]{fig/comp_sbmc/DepthOfFieldTestSynthesizer_13_spp_4/masked_gt.png}
                \\
                DepthOfFieldTestSynthesizer\_13
            \end{tabular}
        \end{adjustbox}
        \hspace{-8.5mm}
        &
        \begin{adjustbox}{valign=t}
        \scriptsize
            \begin{tabular}{ccccc}
                \includegraphics[width=\subghafigsize\textwidth]{fig/comp_sbmc/DepthOfFieldTestSynthesizer_13_spp_4/gt.png} \hspace{\indentspace} &
                \includegraphics[width=\subghafigsize\textwidth]{fig/comp_sbmc/DepthOfFieldTestSynthesizer_13_spp_4/input.png} \hspace{\indentspace} &
                \includegraphics[width=\subghafigsize\textwidth]{fig/comp_sbmc/DepthOfFieldTestSynthesizer_13_spp_4/2011_sen_rpf.png} \hspace{\indentspace} &
                \includegraphics[width=\subghafigsize\textwidth]{fig/comp_sbmc/DepthOfFieldTestSynthesizer_13_spp_4/2012_rousselle_nlm.png} \hspace{\indentspace} &
                \includegraphics[width=\subghafigsize\textwidth]{fig/comp_sbmc/DepthOfFieldTestSynthesizer_13_spp_4/2015_kalantari_lbf.png} 
                \\
                Ground Truth \hspace{\indentspace} &
                4spp\hspace{\indentspace} &
                Sen~\cite{sen2012filtering} \hspace{\indentspace} &
                Rousselle~\cite{rousselle2011adaptive} \hspace{\indentspace} &
                Kalantari~\cite{kalantari2015machine}
                \\
                PSNR$\uparrow$/RelMSE$\downarrow$ \hspace{\indentspace} &
                17.06/1.8784 \hspace{\indentspace} &
                25.29/0.0286 \hspace{\indentspace} &
                28.51/0.0193 \hspace{\indentspace} &
                29.11/0.0165 
                \\
                \includegraphics[width=\subghafigsize\textwidth]{fig/comp_sbmc/DepthOfFieldTestSynthesizer_13_spp_4/2016_bitterli_nfor.png} \hspace{\indentspace} &
                \includegraphics[width=\subghafigsize\textwidth]{fig/comp_sbmc/DepthOfFieldTestSynthesizer_13_spp_4/2017_bako_kpcn.png} \hspace{\indentspace} &
                \includegraphics[width=\subghafigsize\textwidth]{fig/comp_sbmc/DepthOfFieldTestSynthesizer_13_spp_4/disney_samples_ft.png} \hspace{\indentspace} &
                \includegraphics[width=\subghafigsize\textwidth]{fig/comp_sbmc/DepthOfFieldTestSynthesizer_13_spp_4/rmse_multisteps3.png} \hspace{\indentspace} &
                \includegraphics[width=\subghafigsize\textwidth]{fig/comp_sbmc/DepthOfFieldTestSynthesizer_13_spp_4/lr_sp_8_lsp_sp_2x2.png}
                \\ 
                Bitterli~\cite{bitterli2016nonlinearly} \hspace{\indentspace} &
                KPCN~\cite{bako2017kernel} \hspace{\indentspace} &
                KPCN-ft~\cite{bako2017kernel} \hspace{\indentspace} &
                Gharbi~\cite{gharbi2019sample} \hspace{\indentspace} &
                Ours $\times2$
                \\
                29.46/0.0137 \hspace{\indentspace} &
                24.13/0.0647\hspace{\indentspace} &
                24.15/0.0459 \hspace{\indentspace} &
                33.54/\textbf{0.0035} \hspace{\indentspace} &
                \textbf{33.87}/0.0039
                \\
            \end{tabular}
        \end{adjustbox} 
        \\
    \end{tabular}\vspace{-0.15in}
    \caption{
        More visual comparisons on the Gharbi~\cite{gharbi2019sample} dataset.
    }\vspace{-0.1in}
\label{fig:comp_pbrt}
\end{figure*}
